# Supplementary material for: Every Bit Counts in Consensus
Source: arXiv:2306.00431 source file (2023-08-07)
Supplement: Supplementary file 1 [file appendix_C.tex]

\section{Appendix C} 
\label{section:appendix_c}
